# Supplementary material for: Pretraining with Artificial Language: Studying Transferable Knowledge in Language Models
Source: arXiv:2203.10326 source file (2022-03-22)
Supplement: Supplementary file 1 [file mlm-other-languages.tex]

\section{Results from other languages}
\label{appendix:other-languages}

Here we present the result for \cref{sec:tilt-mlm} in Finnish and Japanese in \Figure{fig:tilt-mlm-results-fi} and \ref{fig:tilt-mlm-results-ja}.
The statistics of the dataset are show in \Table{tb:ud-statistics}.

\begin{table}[h]
  \centering
  \begin{tabular}{llrrr} \toprule
  Language & Dataset & \multicolumn{1}{c}{train} & \multicolumn{1}{c}{dev} & \multicolumn{1}{c}{test} \\ \midrule
  English  & EWT     & 16,688                     & 2,741                    & 2,911                     \\
  % Arabic   & NYUAD   & 12575                     & 1579                    & 1580                     \\
  Finnish  & FTB     & 11,502                     & 1,411                    & 1,482                     \\
  Japanese & BCCWJ   & 11,281                     & 2,218                    & 2,074                     \\
  % Korean   & Kaist   & 13956                     & 1226                    & 1366 \\
  \bottomrule
  \end{tabular}
  \caption{The number of sentences in the UD datasets used in the experiment.}
  \label{tb:ud-statistics}
\end{table}

\begin{figure*}[h]

\begin{minipage}{.60\linewidth}
\centering
\subfloat[The results of PoS tagging.]{\label{fig:tili-mlm-pos}\includegraphics[height=4.6cm]{data/tilt_mlm/pos_fi_frozen.png}}
\end{minipage}\hfill
\begin{minipage}{.40\linewidth}
\centering
\subfloat[The results of dependency parsing.]{\label{fig:tili-mlm-dep}\includegraphics[height=4.6cm]{data/tilt_mlm/dep_fi_frozen.png}}
\end{minipage}

\caption{The downstream performance on two syntactic tasks with the Finnish-FTB UD dataset.}
\label{fig:tilt-mlm-results-fi}
\end{figure*}

% \begin{tabular}{lcccccccccc}\toprule
%  & From scratch & Random weights & Uniform & Zipf & Random walk & Zipf Dep-flat & Zipf Dep-nested & English & Spanish & Japanese\\\midrule
%  PoS &  84.3±0.7   &    87.1±0.2    & 85.1±0.6 & 85.3±0.3 &   85.4±0.3  &    85.5±0.6   &     86.7±0.5    & 85.7±0.9 & 86.8±0.4 & 86.4±0.6\\
% Dep & 69.4±1.3   &    60.3±0.6    & 39.4±1.8 & 56.6±0.8 &   57.4±0.9  &    61.9±1.0   &     65.1±1.2    & 61.3±0.9 & 60.9±1.1 & 60.0±1.1\\
% \bottomrule
% \end{tabular}

\begin{figure*}[h]

\begin{minipage}{.60\linewidth}
\centering
\subfloat[The results of PoS tagging.]{\label{fig:tili-mlm-pos}\includegraphics[height=4.6cm]{data/tilt_mlm/pos_ja_frozen.png}}
\end{minipage}\hfill
\begin{minipage}{.40\linewidth}
\centering
\subfloat[The results of dependency parsing.]{\label{fig:tili-mlm-dep}\includegraphics[height=4.6cm]{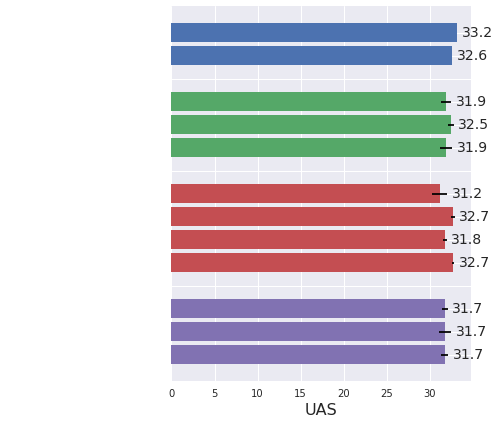}}
\end{minipage}

\caption{The downstream performance on two syntactic tasks with the Japanese-BCCWJ UD dataset.}
\label{fig:tilt-mlm-results-ja}
\end{figure*}

% \begin{tabular}{lcccccccccc}\toprule
% & From scratch & Random weights & Uniform & Zipf & Random walk & Zipf Dep-flat & Zipf Dep-nested & English & Spanish & Japanese\\\midrule
%   PoS & 33.1±0.1   &    29.8±0.2    & 26.8±1.7 & 28.2±0.5 &   29.3±0.3  &    32.5±0.1   &     32.5±0.1    & 31.9±0.7 & 32.5±0.2 & 31.2±1.1 \\
 % & 33.2±0.0   &    32.6±0.0    & 13.8±7.3 & 32.4±0.2 &   32.2±0.3  &    31.9±0.4   &     32.8±0.2    & 32.0±0.8 & 32.4±0.4 & 32.3±0.4 \\
% \bottomrule
% \end{tabular}

Overall, we confirm that we observe similar trend as in English (\cref{sec:tilt-mlm}).
\PoSTagging{} does not seem to require structural knowledge, as indicated by less variance in the performance across pretraining languages.
In Finnish, the \RandomWeights{} baselines even outperforms the model trained from scratch ($84.3\pm0.7$ vs. $87.1\pm0.2$) in this hyper-parameter setting.
Pretraining with the unstructured languages provides lower scores than the \RandomWeights{} baseline overall, confirming the importance of structural knowledge encoded in the pretraining data.

We can also confirm that the \NestingDependency{} outperforms \FlatDependency{} in \DependencyParsing{} ($65.1\pm1.2$ vs. $61.9\pm1.0$ in Finnish, and $32.8\pm0.2$ vs. $31.9\pm0.4$ in Japanese).

Interestingly, in Finnish, the \NestingDependency{} language outperforms natural languages (\English{}, \Spanish{}, \Japanese{}), in contrast with the results from other languages where pretraining with natural languages performs better than \NestingDependency{} in English (\cref{sec:tilt-mlm-results}) and they exhibit comparable performance in the Japanese dataset (\Figure{fig:tilt-mlm-results-ja}).
We leave the investigation of this dataset or language-dependent difference to future work.
